# Supplementary material for: Variational Quantum Linear Solver with Dynamic Ansatz
Source: arXiv:2107.08606 ancillary file (2021-10-31)
Supplement: Supplementary file 1 [file Supplemental_information.pdf]

*Supplemental Information*

# Variational Quantum Linear Solver with Dynamic Ansatz

*Hrushikesh Patil[1], Yulun Wang[2], Predrag Krstic[2]*
[1]Department of Electrical and Computer Engineering, Stony Brook University, Stony Brook, NY 11794
[2] Institute for Advanced Computational Science, Stony Brook University, NY 11794-5250

**Sections and Tables:**

**S1 Generating inputs**
*Table S1*
**S2 Results for dynamic ansatz algorithm with respect to the number of qubits**
*Table S2*
*Table S3*
*Table S4*
**S3 Results for dynamic ansatz algorithm with respect to condition numbers**
*Table S5*
**S4 Results for dynamic ansatz with respect to the sparsity of matrices**
*Table S6*
**S5 Results for dynamic ansatz with respect to the switching number**
*Table S7*
*Table S8*
**S6 Details for Noise Simulation**
**S7 Details for comparison of computational efficiencies of various quantum simulators**
*Table S9*
**S8 Details on the comparison of the effect of number of layers on the TRC and number of iterations**
*Table S10*
**S9 Effect of varying the maximum allowed iterations to the convergence of ADA and ASA**
*Table S11*
*Table S12*
**S10 Comparison of VQLS and classical iterative linear solver**
*Table S13*

**Note**
*In the supplemental Information we present the raw data, explain the choices of the software and discuss in detail the practical implementation of the methods used in the paper. The choice behind using the Pennylane library is ease of switching between different backends, without a need to change the code. In our experiments we found out that the Pennylane with qulacs simulator is the fastest for simulating quantum circuits.*

## S1 Generating inputs

Input matrix A of a SLE needs to be decomposed to a linear combination of unitaries and their coefficients. The input matrix A is of the form of $A = \sum_l c_l P_l$ , where $c_l$ are the complex coefficients and $P_l$ are the unitary matrices. In our experiments, the coefficients are real numbers and the unitaries $P_l$ are simply tensor products of Pauli matrices.

| Number of qubits | Matrix | Coefficients |
|---|---|---|
| 4 | [[0, 0, 0, 0], [2, 2, 0, 2]] | [7, 5.4268] |
| 5 | [[1, 0, 2, 0, 1], [0, 1, 1, 0, 1]] | [2, 1.5505] |
| 6 | [[0, 0, 0, 0, 0, 0], [0, 1, 2, 2, 1, 0]] | [0.2, 0.1899] |
| 8 | [[2, 1, 1, 2, 1, 0, 2, 0]] | [7.0] |

***Table S1*** *Example of matrices and coefficient in decomposed form*

For example, for a SLE with $N = 4$ the $P_l$ is $[X \otimes Z]$. We generate an input matrix A by randomly choosing between gates I, X and Z and placing them on the qubits. The coefficients $c_l$ are chosen randomly. All the matrices and vectors are generated with real coefficients. For experiments which require matrices with certain sparsity, the sparsity is

controlled by generating random matrices until the required sparsity is met. We can also control the condition number scaling by a similar trial-and-error approach. Examples of the matrices in use are given in Table S1.
Here each element in the list represents either one of I, X and Z gates on each of the qubits. “0” stands for I gate, “1” stand for X gate and “2” stands for Z gate. The corresponding matrix can be generated by taking the tensor product of matrices inside the list and then multiplying the matrix with the corresponding coefficient in the coefficient list. For example, the matrix for $N$ = 16 (4 qubits) SLE in table S1 can be written following formula $7(I \otimes I \otimes I \otimes I) + 5.4268(Z \otimes Z \otimes I \otimes Z)$.

For the vector $|b\rangle$ we use a tensor product of Hadamard gates. For example, for a SLE of $N$ = 16 (4 qubits) $|b\rangle = H \otimes H \otimes H \otimes H$. We keep the vector $|b\rangle$ constant irrespective of choice of the matrix A. The reason for the choice is that $|b\rangle$ doesn’t affect the time complexity or the quantum depth of the circuits.

**S2 Results for dynamic ansatz algorithm with respect to the number of qubits**

The Tables S2-S4 contain raw data which, when arithmetically averaged, result in the Table 1 in the paper. The tables on each row contain matrix A of SLE as list of unitaries and their corresponding coefficients followed by the SP input, the final depth, number of optimization iterations and TRCs for ADA and ASA.

| | | ADA | | | | ASA | | |
|---|---|---|---|---|---|---|---|---|
| **Matrix** | **Coefficients** | **SP** | **Final # of Layers** | **Iterations** | **TRC** | **# of layers** | **# of iterations** | **TRC** |
| [[0, 0, 0, 0], [2, 0, 0, 1]] | [-3.0, -1.9365] | 0.01 | 4 | 624 | 1775 | 4 | 303 | 1212 |
| [[0, 0, 0, 0], [1, 1, 0, 0]] | [-4.0, -2.5819] | 0.01 | 2 | 197 | 231 | 4 | 65 | 260 |
| [[0, 0, 0, 0], [1, 1, 2, 1]] | [3.3335, 2.1516] | 0.01 | 4 | 520 | 1301 | 4 | 352 | 1408 |
| [[0, 0, 0, 0], [1, 0, 2, 1]] | [-0.7142, -0.4610] | 0.01 | 4 | 533 | 1343 | 4 | 352 | 1408 |
| [[0, 0, 0, 0], [2, 0, 1, 1]] | [1.0, 0.8386] | 0.01 | 4 | 982 | 3221 | 4 | 1192 | 4768 |
| [[0, 0, 0, 0], [1, 0, 1, 0]] | [2.0, 1.6772] | 0.01 | 2 | 270 | 301 | 4 | 59 | 236 |
| [[0, 0, 0, 0], [2, 2, 0, 0]] | [-1.4285, -1.1980] | 0.01 | 4 | 529 | 1662 | 4 | 369 | 1476 |
| [[0, 0, 0, 0], [0, 0, 1, 1]] | [-5.0, -4.5564] | 0.01 | 2 | 192 | 223 | 4 | 62 | 248 |
| [[0, 0, 0, 0], [0, 2, 2, 1]] | [-0.3333, -0.3037] | 0.01 | 4 | 1167 | 4195 | 4 | 1303 | 5212 |
| [[0, 0, 0, 0], [2, 0, 0, 0]] | [-3.0, -2.7338] | 0.01 | 4 | 1119 | 3526 | 4 | 816 | 3264 |

***Table S2*** *Results for ADA and ASA with 4 qubits*

| **Matrix** | **Coefficients** | **ADA** | | | | **ASA** | | |
|---|---|---|---|---|---|---|---|---|
| | | **SP** | **# of final layers** | **# of iter.** | **TRC** | **# of layers** | **# of iter.** | **TRC** |
| [[0, 0, 0, 0, 0], [1, 1, 2, 2, 0]] | [-0.7143, -0.4093] | 0.001 | 6 | 467 | 1488 | 6 | 109 | 654 |
| [[0, 0, 0, 0, 0], [0, 2, 2, 0, 1]] | [1.0, 0.5730] | 0.001 | 6 | 559 | 1797 | 6 | 127 | 762 |
| [[0, 0, 0, 0, 0], [2, 0, 0, 0, 0]] | [0.8571, 0.4911] | 0.001 | 2 | 262 | 522 | 6 | 78 | 468 |
| [[0, 0, 0, 0, 0], [1, 0, 0, 2, 0]] | [1.2, 0.9303] | 0.001 | 6 | 569 | 2130 | 6 | 260 | 1560 |
| [[0, 0, 0, 0, 0], [1, 0, 2, 1, 0]] | [1.5, 1.1629] | 0.001 | 6 | 568 | 1877 | 6 | 167 | 1002 |
| [[0, 0, 0, 0, 0], [1, 2, 2, 2, 0]] | [1.3333, 1.0336] | 0.001 | 5 | 316 | 1303 | 6 | 217 | 1302 |
| [[0, 0, 0, 0, 0], [1, 2, 2, 1, 1]] | [1.0, 0.7752] | 0.001 | 6 | 698 | 2489 | 6 | 195 | 1170 |
| [[0, 0, 0, 0, 0], [1, 1, 0, 0, 2]] | [-0.2857, -0.2465] | 0.001 | 6 | 794 | 3506 | 6 | 462 | 2772 |
| [[0, 0, 0, 0, 0], [0, 1, 0, 2, 0]] | [0.6, 0.51765] | 0.001 | 6 | 814 | 3641 | 6 | 587 | 3522 |
| [[0, 0, 0, 0, 0], [0, 1, 2, 1, 0]] | [-1.125, -0.9706] | 0.001 | 6 | 683 | 2728 | 6 | 245 | 1470 |
| [[0, 0, 0, 0, 0], [0, 0, 2, 2, 0]] | [-5.0, -4.3138] | 0.001 | 6 | 794 | 3224 | 6 | 324 | 1944 |
| [[0, 0, 0, 0, 0], [1, 0, 2, 1, 0]] | [1.25, 1.1345] | 0.001 | 6 | 760 | 3142 | 6 | 2049 | 12294 |
| [[0, 0, 0, 0, 0], [0, 1, 1, 2, 0]] | [-1.6667, -1.5127] | 0.001 | 6 | 2453 | 13468 | 6 | 3256 | 19536 |
| [[0, 0, 0, 0, 0], [0, 0, 2, 2, 2]] | [-0.8889, -0.8068] | 0.001 | 6 | 587 | 2817 | 6 | 1044 | 6264 |
| [[0, 0, 0, 0, 0], [0, 0, 1, 0, 2]] | [-0.375, -0.3404] | 0.001 | 6 | 1262 | 6337 | 6 | 1238 | 7428 |

***Table S3*** *Results for ADA and ASA with 5 qubits*

| | | ADA | | | | ASA | | |
|---|---|---|---|---|---|---|---|---|
| **Matrix** | **Coefficients** | **SP** | **Final # of Layers** | **Iter.** | **TRC** | **# of layers** | **Iter.** | **TRC** |
| [[0, 2, 1, 2, 2, 1]] | [0.4] | 0.0001 | 6 | 118 | 678 | 8 | 84 | 672 |
| [[0, 0, 0, 0, 0, 0], [2, 1, 0, 1, 0, 0]] | [-1.8, -1.0314] | 0.0001 | 3 | 400 | 1194 | 8 | 131 | 1048 |
| [[0, 0, 0, 0, 0, 0], [2, 1, 0, 2, 2, 2]] | [0.6667, 0.6223] | 0.0001 | 8 | 7199 | 57536 | 8 | 6861 | 54888 |
| [[0, 0, 0, 0, 0, 0], [1, 1, 1, 2, 2, 0]] | [-0.4444, -0.4149] | 0.0001 | 8 | 1991 | 14584 | 8 | 2373 | 18984 |
| [[0, 0, 0, 0, 0, 0], [2, 1, 0, 0, 1, 0]] | [-1.3333, -1.2447] | 0.0001 | 8 | 1919 | 11597 | 8 | 2464 | 19712 |
| [[0, 0, 0, 0, 0, 0], [0, 1, 0, 2, 2, 2]] | [1.25, 1.0784] | 0.0001 | 8 | 662 | 4947 | 8 | 1144 | 9152 |

***Table S4** Results for ADA and ASA with 6 qubits*

## S3 Results for dynamic ansatz algorithm with respect to condition numbers

Table S5 contains raw data for the results presented in Table 2 of the paper. The condition numbers are compared with average of the relative TRCs. In the table S5, considered SLEs are of dimension $N = 32$. Here ARTRCs are calculated with the specified condition numbers. There are 3 more matrices with the exact same TRC values and ARTRC, which we omit from the table to conserve space.

| **Matrix** | **Coefficient** | **Condition Number** | **SP** | **ADA TRC** | **ASA TRC** | **ARTRC** |
|---|---|---|---|---|---|---|
| [[2, 2, 0, 0, 0]] | [0.3333] | 1 | 0.001 | 288 | 270 | 0.0625 |
| [[0, 0, 0, 0, 0], [1, 1, 2, 2, 0]] | [-0.7142, -0.4093] | 3.6840 | 0.001 | 1488 | 654 | 0.560484 |
| [[0, 0, 0, 0, 0], [0, 2, 2, 0, 1]] | [1.0, 0.5730] | 3.6840 | 0.001 | 1797 | 762 | 0.57596 |
| [[0, 0, 0, 0, 0], [2, 0, 0, 0, 0]] | [0.8571, 0.4911] | 3.6840 | 0.001 | 522 | 468 | 0.103448 |
| [[0, 0, 0, 0, 0], [1, 0, 0, 2, 0]] | [1.2, 0.9303] | 7.8995 | 0.001 | 2130 | 1560 | 0.267606 |
| [[0, 0, 0, 0, 0], [1, 0, 2, 1, 0]] | [1.5, 1.1629] | 7.8995 | 0.001 | 1877 | 1002 | 0.466169 |
| [[0, 0, 0, 0, 0], [1, 2, 2, 2, 0]] | [1.3333, 1.0337] | 7.8995 | 0.001 | 1303 | 1302 | 0.000767 |
| [[0, 0, 0, 0, 0], [1, 2, 2, 1, 1]] | [1.0, 0.7752] | 7.8995 | 0.001 | 2489 | 1170 | 0.529932 |
| [[0, 0, 0, 0, 0], [1, 1, 0, 0, 2]] | [-0.2857, -0.2465] | 13.5720 | 0.001 | 3506 | 2772 | 0.209355 |
| [[0, 0, 0, 0, 0], [0, 1, 0, 2, 0]] | [0.6, 0.5177] | 13.5720 | 0.001 | 3641 | 3522 | 0.032683 |
| [[0, 0, 0, 0, 0], [0, 1, 2, 1, 0]] | [-1.125, -0.9706] | 13.5720 | 0.001 | 2728 | 1470 | 0.461144 |
| [[0, 0, 0, 0, 0], [0, 0, 2, 2, 0]] | [-5.0, -4.3136] | 13.5720 | 0.001 | 3224 | 1944 | 0.397022 |
| [[0, 0, 0, 0, 0], [1, 0, 2, 1, 0]] | [1.25, 1.1345] | 20.6519 | 0.001 | 3142 | 12294 | -2.91279 |
| [[0, 0, 0, 0, 0], [0, 1, 1, 2, 0]] | [-1.6667, -1.5127] | 20.6519 | 0.001 | 13468 | 19536 | -0.45055 |
| [[0, 0, 0, 0, 0], [0, 0, 2, 2, 2]] | [-0.8888, -0.8067] | 20.6519 | 0.001 | 2817 | 6264 | -1.22364 |
| [[0, 0, 0, 0, 0], [0, 0, 1, 0, 2]] | [-0.375, -0.3404] | 20.6519 | 0.001 | 6337 | 7428 | -0.17216 |

***Table S5** Results for the comparison of the ADA and ASA TRCs when condition number changes.*

## S4 Results for dynamic ansatz with respect to the sparsity of matrices

Table S6 contains raw data for the comparison of the TRCs of ADA and ASA vs sparsity of the matrices (see also Table 3 in the paper). Here the number of qubits were 4 and ARTRC was calculated and averaged over. One important thing to note is that there are 9 more matrices with exact same results for sparsity 0.9375.

| Matrix | Coefficient | Sparsity | SP | ADA | | ASA | | ARTRC |
|---|---|---|---|---|---|---|---|---|
| | | | | Iter. | TRC | Iter. | TRC | |
| [[1, 1, 1, 0], [2, 2, 2, 1], [1, 2, 2, 0], [0, 1, 0, 1]] | [0.8, 2.0, 3.0, 1.6667] | 0.75 | 0.005 | 310 | 649 | 143 | 572 | 0.1346 |
| [[2, 2, 0, 1], [2, 1, 0, 2], [0, 2, 0, 2], [1, 0, 1, 2]] | [0.875, 3.0, 1.25, 2.25] | 0.75 | 0.005 | 107 | 130 | 41 | 164 | -0.2073 |
| [[2, 2, 0, 1], [2, 1, 1, 2], [1, 1, 1, 0], [0, 2, 1, 0]] | [0.25, 7.0, 0.888, 0.875] | 0.75 | 0.005 | 149 | 196 | 56 | 224 | -0.125 |
| [[1, 1, 2, 1], [1, 2, 2, 0], [0, 1, 2, 1], [1, 1, 2, 2]] | [0.7778, 1.0, 0.6, 0.1111] | 0.75 | 0.005 | 148 | 165 | 36 | 144 | 0.1458 |
| [[2, 0, 0, 0], [1, 2, 1, 1], [0, 0, 1, 2], [1, 0, 2, 0]] | [2.0, 1.0, 1.25, 9.0] | 0.75 | 0.005 | 179 | 244 | 80 | 320 | -0.2375 |
| [[1, 1, 1, 0], [1, 0, 0, 2], [1, 1, 2, 1], [2, 0, 2, 0]] | [0.3, 0.7778, 0.75, 1.0] | 0.75 | 0.005 | 304 | 601 | 129 | 516 | 0.1647 |
| [[2, 0, 2, 1], [2, 0, 0, 0], [1, 1, 1, 1]] | [8.0, 0.8334, 1.125] | 0.8125 | 0.005 | 173 | 223 | 60 | 240 | -0.0708 |
| [[0, 0, 0, 1], [1, 2, 1, 0], [0, 2, 0, 2]] | [0.3333, 1.0, 9.0] | 0.8125 | 0.005 | 152 | 198 | 55 | 220 | -0.1 |
| [[1, 1, 0, 0], [1, 2, 2, 0], [1, 2, 0, 1]] | [6.0, 0.3333, 0.5] | 0.8125 | 0.005 | 151 | 185 | 49 | 196 | -0.0561 |
| [[1, 1, 2, 0], [1, 0, 0, 0], [2, 1, 2, 0]] | [7.0, 1.0, 8.0] | 0.8125 | 0.005 | 169 | 198 | 42 | 168 | 0.1785 |
| [[1, 2, 0, 1], [0, 1, 0, 1], [2, 1, 2, 2]] | [0.5, 2.6665, 0.4] | 0.8125 | 0.005 | 156 | 188 | 47 | 188 | 0 |
| [[2, 0, 1, 1], [1, 1, 0, 2], [2, 2, 1, 0]] | [0.5, 0.75, 9.0] | 0.8125 | 0.005 | 172 | 212 | 53 | 212 | 0 |
| [[1, 2, 2, 0], [2, 1, 1, 0], [2, 1, 2, 2]] | [0.3, 1.25, 0.3333] | 0.8125 | 0.005 | 155 | 221 | 68 | 272 | -0.1875 |
| [[1, 1, 1, 1], [1, 0, 1, 0], [1, 0, 2, 0]] | [1.4285, 0.71, 1.6667] | 0.8125 | 0.005 | 143 | 166 | 32 | 128 | 0.2968 |
| [[2, 1, 0, 0], [2, 2, 2, 0], [1, 0, 0, 1]] | [2.6665, 8.0, 5.0] | 0.8125 | 0.005 | 205 | 319 | 97 | 388 | -0.1778 |
| [[2, 1, 0, 2], [1, 1, 1, 2]] | [0.4, 0.3] | 0.875 | 0.005 | 167 | 190 | 37 | 148 | 0.2837 |
| [[1, 0, 0, 1], [1, 1, 2, 1]] | [0.75, 6.0] | 0.875 | 0.005 | 158 | 206 | 57 | 228 | -0.0964 |
| [[2, 2, 1, 2], [2, 0, 2, 2]] | [2.0, 2.5] | 0.875 | 0.005 | 430 | 1185 | 169 | 676 | 0.7529 |
| [[1, 2, 1, 2], [0, 2, 1, 1]] | [3.0, 1.2857] | 0.875 | 0.005 | 181 | 205 | 40 | 160 | 0.2812 |
| [[2, 1, 1, 2], [2, 2, 1, 1]] | [4.5, 1.125] | 0.875 | 0.005 | 194 | 242 | 67 | 268 | -0.097 |
| [[1, 0, 0, 1], [2, 0, 1, 1]] | [2.5, 10.0] | 0.875 | 0.005 | 178 | 202 | 43 | 172 | 0.1744 |
| [[2, 0, 1, 1], [2, 2, 2, 1]] | [0.3333, 1.1429] | 0.875 | 0.005 | 166 | 240 | 73 | 292 | -0.1780 |
| [[1, 1, 2, 2], [1, 2, 2, 2]] | [0.6667, 1.0] | 0.875 | 0.005 | 169 | 192 | 38 | 152 | 0.2631 |
| [[1, 2, 1, 0]] | [1.3333] | 0.9375 | 0.005 | 161 | 195 | 51 | 204 | -0.0441 |

***Table S6** Results for ADA and ASA with change of sparsity*

## S5 Results for dynamic ansatz with respect to the switching number

The table S7 contains the raw data for ADA with *SP* = 0.1, 0.01, 0.001, 0.00001 and for ASA. The number of qubits is 4 and the maximum number of layers is 4. Table S8 has the raw data for final layers of the ADA.

| Matrix | Coefficient | ADA TRC | | | | ASA TRC |
|---|---|---|---|---|---|---|
| | | SP = 0.1 | SP = 0.01 | SP = 0.001 | SP = 0.00001 | |
| [[1, 2, 0, 2]] | [0.7142] | 1796 | 1796 | 1576 | 1671 | 1804 |
| [[2, 1, 1, 2]] | [0.75] | 1796 | 1796 | 1576 | 1671 | 1804 |
| [[0, 2, 2, 2]] | [4.0] | 1796 | 1796 | 1576 | 1671 | 1804 |
| [[2, 0, 0, 1]] | [1.0] | 1796 | 1796 | 1576 | 1671 | 1804 |
| [[2, 1, 2, 2]] | [4.0] | 1796 | 1796 | 1576 | 1671 | 1804 |
| [[0, 2, 1, 2]] | [0.125] | 1796 | 1796 | 1576 | 1671 | 1804 |
| [[1, 1, 2, 2]] | [1.75] | 1796 | 1796 | 1576 | 1671 | 1804 |
| [[0, 0, 1, 1]] | [0.75] | 1796 | 1796 | 1576 | 1671 | 1804 |
| [[2, 1, 1, 1]] | [9.0] | 1796 | 1796 | 1576 | 1671 | 1804 |
| [[0, 0, 2, 1]] | [1.3333] | 1796 | 1796 | 1576 | 1671 | 1804 |
| [[0, 0, 0, 0], [0, 0, 0, 0]] | [-1.2857, -0.7367] | 1796 | 1796 | 1576 | 1671 | 1804 |
| [[0, 0, 0, 0], [2, 2, 1, 0]] | [-0.5, -0.2865] | 5528 | 5528 | 9666 | 9998 | 5544 |
| [[0, 0, 0, 0], [0, 1, 0, 1]] | [-0.1666, -0.0955] | 1260 | 2339 | 1421 | 1421 | 1268 |
| [[0, 0, 0, 0], [2, 0, 2, 2]] | [2.0, 1.1460] | 3608 | 3608 | 5673 | 4842 | 3612 |
| [[0, 0, 0, 0], [1, 1, 0, 1]] | [-1.6666, -1.2921] | 1024 | 1704 | 1035 | 1149 | 1032 |
| [[0, 0, 0, 0], [1, 2, 2, 2]] | [-3.0, -2.3258] | 15992 | 15992 | 15992 | 9998 | 16004 |
| [[0, 0, 0, 0], [2, 0, 0, 0]] | [-0.6, -0.4651] | 6272 | 6272 | 9239 | 9998 | 6276 |
| [[0, 0, 0, 0], [1, 1, 0, 2]] | [-0.8, -0.6202] | 14008 | 11581 | 10400 | 9998 | 14108 |
| [[0, 0, 0, 0], [2, 1, 0, 1]] | [-0.7, -0.5426] | 8472 | 8600 | 10536 | 9998 | 8484 |
| [[0, 0, 0, 0], [0, 0, 0, 1]] | [-10.0, -8.6275] | 1256 | 2242 | 1555 | 1555 | 1264 |
| [[0, 0, 0, 0], [1, 1, 1, 2]] | [0.625, 0.5392] | 15992 | 15822 | 12745 | 9998 | 16004 |

***Table S7*** *TRC data for SP parameter comparison (21 trials)*

| Matrix | Coefficient | ADA Final Layers | | | | ASA Final Layers |
|---|---|---|---|---|---|---|
| | | SP = 0.1 | SP = 0.01 | SP = 0.001 | SP = 0.00001 | |
| [[1, 2, 0, 2]] | [0.7142] | 4 | 4 | 2 | 2 | 4 |
| [[2, 1, 1, 2]] | [0.75] | 4 | 4 | 2 | 2 | 4 |
| [[0, 2, 2, 2]] | [4.0] | 4 | 4 | 2 | 2 | 4 |
| [[2, 0, 0, 1]] | [1.0] | 4 | 4 | 2 | 2 | 4 |
| [[2, 1, 2, 2]] | [4.0] | 4 | 4 | 2 | 2 | 4 |
| [[0, 2, 1, 2]] | [0.125] | 4 | 4 | 2 | 2 | 4 |
| [[1, 1, 2, 2]] | [1.75] | 4 | 4 | 2 | 2 | 4 |
| [[0, 0, 1, 1]] | [0.75] | 4 | 4 | 2 | 2 | 4 |
| [[2, 1, 1, 1]] | [9.0] | 4 | 4 | 2 | 2 | 4 |
| [[0, 0, 2, 1]] | [1.3333] | 4 | 4 | 2 | 2 | 4 |
| [[0, 0, 0, 0], [0, 0, 0, 0]] | [-1.2857, -0.7367] | 4 | 4 | 2 | 2 | 4 |
| [[0, 0, 0, 0], [2, 2, 1, 0]] | [-0.5, -0.2865] | 4 | 4 | 4 | 4 | 4 |
| [[0, 0, 0, 0], [0, 1, 0, 1]] | [-0.1666, -0.0955] | 4 | 4 | 2 | 2 | 4 |
| [[0, 0, 0, 0], [2, 0, 2, 2]] | [2.0, 1.1460] | 4 | 4 | 4 | 3 | 4 |
| [[0, 0, 0, 0], [1, 1, 0, 1]] | [-1.6666, -1.2921] | 4 | 4 | 2 | 2 | 4 |
| [[0, 0, 0, 0], [1, 2, 2, 2]] | [-3.0, -2.3258] | 4 | 4 | 4 | 4 | 4 |
| [[0, 0, 0, 0], [2, 0, 0, 0]] | [-0.6, -0.4651] | 4 | 4 | 4 | 4 | 4 |
| [[0, 0, 0, 0], [1, 1, 0, 2]] | [-0.8, -0.6202] | 4 | 4 | 4 | 4 | 4 |
| [[0, 0, 0, 0], [2, 1, 0, 1]] | [-0.7, -0.5426] | 4 | 4 | 4 | 4 | 4 |
| [[0, 0, 0, 0], [0, 0, 0, 1]] | [-10.0, -8.6275] | 4 | 4 | 2 | 2 | 4 |
| [[0, 0, 0, 0], [1, 1, 1, 2]] | [0.625, 0.5392] | 4 | 4 | 4 | 4 | 4 |

***Table S8*** *Final depth data for the SP parameter comparison for 21 trials.*

## S6 Details for Noise Simulation

The depolarizing error is defined by the depolarization channel: $\varepsilon(\rho) = (1-p)\rho + p\frac{I}{2^n}$ where ρ represents the density operator of initial state, *p* is the probability of depolarization, $\frac{I}{2^n}$ is completely mixed state density, and *n* is the number of qubits in the error channel [1]. Thermal relaxation error is defined with relaxation times of individual qubits with $T_1$ and $T_2$ parameters and the gate time of the actual device, in our case the device is "*ibm_16_melbourne*". $T_1$ and $T_2$ in our noise model have an average value of 56.54 ns and 55.3 ns for all qubits. The average error probability in backend is 0.02090 for single gate and 0.03809 for CNOT gate. The readout error records the probability that the classical bit value is flipped from the true outcome after a measurement. The probability of readout error is set to 0.045 in our simulator, reference [2] in the paper.

## S7 Details for comparison of computational efficiencies of various quantum simulators

The backends used are Pennylane-qiskit, the default Pennylane simulator and the Pennylane-qulacs simulator. With these backends we measured the time taken by the cost function evaluation $t_C$ and the time taken by the classical optimization loop $t_L$ **.** We check for the best (i.e., the fastest) simulator for our experiments. Small $t_C$ and $t_L$ indicates that our VQLS ADA and ASA simulations will complete with much lesser time. The results are presented in Table S9.

| **Qubits** | **Layers** | **Pennylane-Qulacs** | | **Pennylane-default** | | **Pennylane-qiskit** | |
|---|---|---|---|---|---|---|---|
| | | $t_C$ | $t_L$ | $t_C$ | $t_L$ | $t_C$ | $t_L$ |
| 8 | 8 | 0.1288 | 15.3294 | 0.2586 | 32.2262 | 0.4905 | 60.535 |
| 8 | 16 | 0.2395 | 53.116 | 0.4187 | 105.0125 | 0.6745 | 164.0519 |
| 8 | 32 | 0.4417 | 196.1767 | 0.7172 | 360.0926 | 1.0283 | 505.6825 |
| 6 | 12 | 0.0382 | 3.3295 | 0.0747 | 6.3007 | 0.6068 | 58.5634 |
| 6 | 8 | 0.0281 | 1.8623 | 0.0548 | 3.2233 | 0.3747 | 33.7188 |

***Table S9*** *Comparison of quantum simulator based on time taken to calculate a single cost function ( $t_c$ ) and the loop time ( $t_l$ ) s. The unit of time is second.*

## S8 Details on the comparison of the effect of number of layers on the TRC and number of iterations

Size of SLEs were $N$ = 256 and 21 systems were solved with ADA, ASA here ADA, with $d_{min}$ = 8 and ASA with $d_{min}$ = 16. Of 21 systems, 6 SLEs reached convergence for all 3 combinations (18 trials all together).

| **ADA** | | | **ASA (layers = 8)** | | | **ASA (layers = 16)** | | |
|---|---|---|---|---|---|---|---|---|
| **Final layers** | **Iterations** | **TRC** | **Final # of layers** | **Iterations** | **TRC** | **# of layers** | **Iterations** | **TRC** |
| 8 | 1863 | 14848 | 8 | 1857 | 14856 | 16 | 905 | 14480 |
| 8 | 1863 | 14848 | 8 | 1857 | 14856 | 16 | 905 | 14480 |
| 8 | 1863 | 14848 | 8 | 1857 | 14856 | 16 | 905 | 14480 |
| 8 | 1863 | 14848 | 8 | 1857 | 14856 | 16 | 905 | 14480 |
| 8 | 2488 | 19848 | 8 | 2482 | 19856 | 16 | 1235 | 19760 |
| 8 | 2998 | 23928 | 8 | 2991 | 23928 | 16 | 1451 | 23216 |

***Table S10*** *Comparison of ADA, ASA with number of layers 8 and 16*

## S9 Effect of varying the maximum allowed iterations to the convergence of ADA and ASA

| | | | Max iterations = 24000 | | Max iterations = 4000 | |
|---|---|---|---|---|---|---|
| Matrix | Coeff | Condition Number | Dynamic | Static | Dynamic | Static |
| | | | Converged? | Converged? | Converged? | Converged? |
| [[0, 1, 1, 1]] | [3.0] | 1 | TRUE | TRUE | TRUE | TRUE |
| [[0, 0, 1, 2]] | [1.14] | 1 | TRUE | TRUE | TRUE | TRUE |
| [[2, 1, 1, 1]] | [0.25] | 1 | TRUE | TRUE | TRUE | TRUE |
| [[0, 0, 2, 2]] | [1.25] | 1 | TRUE | TRUE | TRUE | TRUE |
| [[2, 0, 0, 1]] | [0.71] | 1 | TRUE | TRUE | TRUE | TRUE |
| [[1, 1, 1, 1]] | [0.5] | 1 | TRUE | TRUE | TRUE | TRUE |
| [[2, 1, 0, 2]] | [1.5] | 1 | TRUE | TRUE | TRUE | TRUE |
| [[2, 2, 1, 2]] | [0.3] | 1 | TRUE | TRUE | TRUE | TRUE |
| [[2, 2, 1, 2]] | [1.0] | 1 | TRUE | TRUE | TRUE | TRUE |
| [[1, 0, 1, 2]] | [0.84] | 1 | TRUE | TRUE | TRUE | TRUE |
| [[0, 0, 0, 0], [0, 2, 1, 2]] | [-0.875, -0.50] | 3.684031 | FALSE | FALSE | FALSE | FALSE |
| [[0, 0, 0, 0], [2, 1, 0, 1]] | [-0.75, -0.43] | 3.684031 | TRUE | TRUE | TRUE | TRUE |
| [[0, 0, 0, 0], [1, 1, 2, 1]] | [-1.33, -0.76] | 3.684031 | TRUE | TRUE | TRUE | TRUE |
| [[0, 0, 0, 0], [0, 2, 1, 1]] | [2.0, 1.14] | 3.684031 | TRUE | TRUE | TRUE | TRUE |
| [[0, 0, 0, 0], [2, 1, 2, 0]] | [-1.25, -0.97] | 7.89953 | FALSE | FALSE | FALSE | FALSE |
| [[0, 0, 0, 0], [0, 2, 2, 2]] | [-0.75, -0.58] | 7.89953 | TRUE | TRUE | TRUE | TRUE |
| [[0, 0, 0, 0], [2, 2, 2, 0]] | [0.33, 0.25] | 7.89953 | TRUE | TRUE | TRUE | TRUE |
| [[0, 0, 0, 0], [2, 1, 0, 2]] | [1.5, 1.16] | 7.89953 | TRUE | TRUE | TRUE | TRUE |
| [[0, 0, 0, 0], [1, 2, 0, 1]] | [-0.125, -0.09] | 7.89953 | TRUE | TRUE | TRUE | TRUE |
| [[0, 0, 0, 0], [2, 1, 1, 2]] | [-0.28, -0.24] | 13.57209 | TRUE | TRUE | TRUE | TRUE |
| [[0, 0, 0, 0], [2, 2, 0, 2]] | [-2.67, -2.30] | 13.57209 | TRUE | TRUE | TRUE | TRUE |
| [[0, 0, 0, 0], [1, 1, 0, 0]] | [-1.28, -1.10] | 13.57209 | TRUE | TRUE | TRUE | TRUE |
| [[0, 0, 0, 0], [0, 0, 0, 1]] | [1.0, 0.86] | 13.57209 | TRUE | TRUE | TRUE | TRUE |
| [[0, 0, 0, 0], [0, 2, 1, 0]] | [4.0, 3.63] | 20.652 | TRUE | TRUE | TRUE | TRUE |
| [[0, 0, 0, 0], [0, 2, 0, 2]] | [1.25, 1.13] | 20.652 | FALSE | FALSE | FALSE | FALSE |
| [[0, 0, 0, 0], [1, 2, 1, 0]] | [-7.0, -6.35] | 20.652 | TRUE | TRUE | TRUE | TRUE |
| [[0, 0, 0, 0], [0, 2, 1, 0]] | [-3.5, -3.17] | 20.652 | TRUE | TRUE | TRUE | TRUE |
| [[0, 0, 0, 0], [2, 1, 2, 2]] | [-1.0, -0.90] | 20.652 | FALSE | FALSE | FALSE | FALSE |
| [[0, 0, 0, 0], [0, 2, 2, 1]] | [-0.11, -0.10] | 29.10 | TRUE | FALSE | TRUE | FALSE |
| [[0, 0, 0, 0], [1, 1, 2, 1]] | [0.56, 0.52] | 29.10 | TRUE | FALSE | TRUE | FALSE |
| [[0, 0, 0, 0], [2, 2, 2, 0]] | [2.0, 1.862] | 29.10 | TRUE | TRUE | TRUE | TRUE |
| [[0, 0, 0, 0], [1, 2, 1, 1]] | [1.0, 0.93] | 29.10212 | TRUE | FALSE | TRUE | FALSE |
| [[0, 0, 0, 0], [1, 2, 0, 1]] | [-0.57, -0.53] | 29.10212 | TRUE | TRUE | TRUE | FALSE |
| [[0, 0, 0, 0], [0, 2, 0, 2]] | [5.0, 4.75] | 38.89292 | FALSE | FALSE | FALSE | FALSE |
| [[0, 0, 0, 0], [0, 0, 1, 2]] | [0.9, 0.85] | 38.89292 | TRUE | TRUE | FALSE | FALSE |
| [[0, 0, 0, 0], [1, 2, 2, 2]] | [-0.71, -0.67] | 38.89292 | FALSE | FALSE | FALSE | FALSE |
| [[0, 0, 0, 0], [2, 0, 2, 0]] | [-0.14, -0.13] | 38.89292 | FALSE | FALSE | FALSE | FALSE |
| [[0, 0, 0, 0], [2, 1, 2, 0]] | [-1.8, -1.71] | 38.89292 | FALSE | FALSE | FALSE | FALSE |
| [[0, 0, 0, 0], [0, 1, 0, 2]] | [2.25, 2.16] | 50 | TRUE | TRUE | FALSE | FALSE |

***Table S11*** *Effect of varying the maximum allowable iterations on the convergence of ADA and ASA VQLS*

Almost 50% of the systems (considering all experiments including 5, 6 qubit LSE) did not converge because of the limit we applied to the maximum number of iterations. Our runs were limited to 4000 iterations in case of the 4-qubit systems, 6000 for the 5-qubit, 12000 for the 6-qubit, and 38400 for the 8-qubit systems. The rationale behind limiting the maximum number of iterations was the large amount of time required to simulate quantum circuits on a classical computer. An important factor affecting the simulation time is a choice of the optimization strategy. The largest time is consumed by the gradient calculations, which is done in the quantum part of our algorithm. The ratio of the cost function calculation and a single optimization step is 1:2p where p is the number of parameters. To demonstrate that VQLS can converge when increasing the maximum number of iterations, we performed a series of experiments to explore the convergence characteristics of the 4-qubit LSE systems with maximum number of iterations 4000 and

24000. We observed an increase in number of converged cases (upto 82%) when we increased the maximum number of iterations.

| Matrix | Coeff | Condition Number | Dynamic | | | | Static | | | |
|---|---|---|---|---|---|---|---|---|---|---|
| | | | Depth | Iter | TRC | Converged? | Depth | Iter | TRC | Converged? |
| [[0, 0, 0, 0], [0, 2, 2, 1]] | [-0.11, -0.10] | 29.10212 | 4 | 9182 | 36415 | TRUE | 4 | 24001 | 96004 | FALSE |
| [[0, 0, 0, 0], [1, 1, 2, 1]] | [0.56, 0.51] | 29.10212 | 4 | 1885 | 7099 | TRUE | 4 | 24001 | 96004 | FALSE |
| [[0, 0, 0, 0], [1, 2, 1, 1]] | [1.0, 0.93] | 29.10212 | 4 | 1885 | 7099 | TRUE | 4 | 24001 | 96004 | FALSE |

***Table S12:*** *Cases where ADA converges but ASA failed to converge for maximum iterations = 24000 and qubits n = 4 (N = 16)*

## S10 Comparison of VQLS and classical iterative linear solver:

| | Conjugate Gradient [3] | HHL [3] | VQLS [4] |
|---|---|---|---|
| Runtime complexity | $\mathrm{O}\left(Ns\kappa\log(1/\varepsilon)\right)$ | $\mathrm{O}\left(s^2\frac{\kappa^2}{\varepsilon}\log_2 N\right)$ | $\mathrm{O}\left((\log_2 N)^{8.5}\kappa\log(1/\varepsilon)\right)$ |

***Table S13****: Comparison of Conjugate Gradient, HHL and VQLS. N is the system size, s is the sparsity, κ is the condition number and ε is the precision.*

The original VQLS has polylogarithmic scaling with N, linear scaling with the condition number and logarithmic scaling in precision (Table S13). The scaling is similar for the fully-quantum algorithm HHL in terms of condition number and precision. Since VQLS has polylogarithmic scaling with N, iterative classical methods are faster for lower sizes, and advantage is expected for very large system sizes, much beyond the 8-qubit considered in this study.

## References


[1] M. A. Nielsen and I. L. Chuang, Quantum Computation and Quantum Information: 10th Anniversary Edition, (Cambridge University Press, USA, 2011).
[2] G. Aleksandrowicz et al., "Qiskit: An Open-source Framework for Quantum Computing," (2019), https://doi.org/10.5281/zenodo.2562111.
[3] A. W. Harrow, A. Hassidim, and S. Lloyd, Quantum algorithm for linear systems of equations, Phys. Rev. Lett.103, 150502 (2009).
[4] C. Bravo-Prieto, R. LaRose, M. Cerezo, Y. Subasi, L. Cincio, and P. J. Coles, Variational quantum linear solver (2020), arXiv:1909.05820 [quant-ph].
